# Supplementary material for: Stochastic Ordering of Interferences in Large-scale Wireless Networks
Source: arXiv:1204.6341 source file (2012-10-24)
Supplement: Supplementary file 1 [file appendix_Proof_for_Lt_PPP.tex]

\label{app:Lt_PPP}
Let $X$ be a non-negative random variable, with ${\mu_j}_{j=0}^{\infty}$ its infinite sequence of ordinary moments which characterize $X$. The fractional moment $\mathbb{E}[x^{\alpha}], \alpha > 0$ can be expressed by means of Laplace transform $\mathcal{L}_{X}(s)$ and the ordinary moments as follows \cite{Inverardia2005}:
\begin{equation}
\label{eqn:Lt_PPP_1}
\mathbb{E}[X^{\alpha+M-1}]=(-1)^M\frac{\prod_{j=0}^{M-1}(\alpha+j)}{\Gamma(1-\alpha)}\int_{0}^{\infty}s^{-\alpha-M}\left[\mathcal{L}_{X}(s)-\sum_{j=0}^{M-1}(-1)^{j}\frac{\mu_j s^j}{j!}\right]\mathrm{d}s
\end{equation}
with $M=1,2,\dots$ and $\alpha \in (0,1)$.

When $M=1$, from \eqref{eqn:Lt_PPP_1} with $h_{I_1} \leq_{\mathrm{Lt}} h_{I_2}$ we have the following equation
\begin{equation}
\label{eqn:Lt_PPP_2}
\mathbb{E}[h_{I_1}^{\alpha}] - \mathbb{E}[h_{I_2}^{\alpha}] = -\frac{\alpha}{\Gamma(1-\alpha)}\int_{0}^{\infty}s^{-\alpha-1}\left[\mathcal{L}_{h_{I_1}}(s)-\mathcal{L}_{h_{I_2}}(s)\right]\mathrm{d}s \leq 0
\end{equation}
since $\frac{\alpha}{\Gamma[1-\alpha]} \geq 0$ and $\mathcal{L}_{h_{I_1}}(s) \geq \mathcal{L}_{h_{I_2}}(s)$ from LT ordering between $h_{I_1}$ and $h_{I_2}$. Therefore, if $h_{I_1} \leq_{\mathrm{Lt}} h_{I_2}$, then Theorem \ref{Lt_ordering_w_fading_for_PPP} is followed by $\mathbb{E}[h_{I_1}^{\alpha}] \leq \mathbb{E}[h_{I_2}^{\alpha}]$.
