# Supplementary material for: Stochastic Ordering of Interferences in Large-scale Wireless Networks
Source: arXiv:1204.6341 source file (2012-10-24)
Supplement: Supplementary file 2 [file appendix_Proof_for_preserving_ordering.tex]

\label{app:Preservation_of_Lf_ordering}
With the Laplace functional of marked point process \cite{Daley2003}, we can establish as follows:
\begin{eqnarray}
\label{eqn:proof_preserving_ordering_1}
L_{\widetilde{\Phi}}(u)&=&\mathbb{E}_{\Phi}\left[\prod_{x\in\Phi}\int_{\mathbb{R}^{+}}\exp(-\kappa u(x))f(\kappa)\mathrm{d}\kappa\right] \\
\label{eqn:proof_preserving_ordering_2}
&=&\mathbb{E}_{\Phi}\left[\prod_{x\in\Phi}\exp\left(-\left(-\log\int_{\mathbb{R}^{+}}\exp\left(-\kappa u(x)\right)f(\kappa)\mathrm{d}\kappa\right)\right)\right] \\
\label{eqn:proof_preserving_ordering_3}
&=&\mathbb{E}_{\Phi}\left[\prod_{x\in\Phi}\exp\left(-\tilde{u}(x)\right)\right]
=\mathbb{E}_{\Phi}\left[\exp\left(-\sum_{x\in\Phi}\tilde{u}(x)\right)\right]
\end{eqnarray}
where $\tilde{u}(x)=-\log\int_{\mathbb{R}^{+}}\exp\left(-\kappa u(x)\right)f(\kappa)\mathrm{d}\kappa$. Since $0 \leq \int_{\mathbb{R}^{+}}\exp\left(-\kappa u(x)\right)f(\kappa)\mathrm{d}\kappa \leq 1$, $\tilde{u}(x)$ is a non-negative function of $x$. From \eqref{eqn:proof_preserving_ordering_3}, the Laplace functional of marked point process can be expressed as follows:
\begin{equation}
\label{eqn:Lf_marked_pp}
L_{\widetilde{\Phi}}(u)=L_{\Phi}(\tilde{u}) \text{.}
\end{equation}
Therefore, from \eqref{eqn:Lf_marked_pp} and the definition of LF ordering in \eqref{eqn:Def_Lf_ordering}, if $\Phi_1 \leq_{\mathrm{Lf}} \Phi_2$, then $\widetilde{\Phi}_1 \leq_{\mathrm{Lf}} \widetilde{\Phi}_2$.
