# Supplementary material for: Stochastic Ordering of Interferences in Large-scale Wireless Networks
Source: arXiv:1204.6341 source file (2012-10-24)
Supplement: Supplementary file 3 [file appendix_Proof_for_Lt_ordering_marked_PP.tex]

\label{app:Lt_ordering_marked_PP}
The Laplace functional of marked point process $\widetilde{\Phi}$ with independently marking $h_I$ can be expressed as follows \cite{Daley2003}:
\begin{equation}
\label{eqn:proof_Lt_ordering_marked_PP_1}
L_{\widetilde{\Phi}}(u)=\mathbb{E}_{\Phi}\left[\prod_{x\in\Phi}\int_{\mathbb{R}^{+}}\exp(-u(x,h_I))F(\mathrm{d}h_I\vert x)\right]
\end{equation}
If the process is stationary, the mark kernel is independent of $x$, $F(\cdot\vert x)=F(\cdot)$. Then, with $u(x,h_I)=sh_I g(x)$, the Laplace transform of interference in the presence of fading $h_I$ can be expressed as follows:
\begin{eqnarray}
\label{eqn:proof_Lt_ordering_marked_PP_2}
\mathcal{L}_{I_{\widetilde{\Phi}}}(s)&=&\mathbb{E}_{\Phi}\left[\prod_{x\in\Phi}\int_{\mathbb{R}^{+}}\exp(-sh_I g(x))f(h_I)\mathrm{d}h_I\right] \\
\label{eqn:proof_Lt_ordering_marked_PP_3}
&=&\mathbb{E}_{\Phi}\left[\prod_{x\in\Phi}\exp\left(-\left(-\log\int_{\mathbb{R}^{+}}\exp\left(-sh_I g(x)\right)f(h_I)\mathrm{d}h_I\right)\right)\right] \\
\label{eqn:proof_Lt_ordering_marked_PP_4}
&=&\mathbb{E}_{\Phi}\left[\prod_{x\in\Phi}\exp\left(-\tilde{u}(x)\right)\right]
=\mathbb{E}_{\Phi}\left[\exp\left(-\sum_{x\in\Phi}\tilde{u}(x)\right)\right]
\end{eqnarray}
where $\tilde{u}(x)=-\log\int_{\mathbb{R}^{+}}\exp\left(-sh_Ig(x)\right)f(h_I)\mathrm{d}h_I$. Since $0 \leq \int_{\mathbb{R}^{+}}\exp\left(-sh_Ig(x)\right)f(h_I)\mathrm{d}h_I \leq 1$ which is the Laplace transform of $h_I$ evaluated at $sg(x)$, $\tilde{u}(x)$ is a nonnegative function of $x$. Therefore, from the definition of LF ordering in \eqref{eqn:Def_Lf_ordering}, if $\Phi_1 \leq_{\mathrm{Lf}} \Phi_2$, then $I_{\widetilde{\Phi}_1} \leq_{\mathrm{Lt}} I_{\widetilde{\Phi}_2}$.
